# Supplementary material for: Federated Reinforcement Learning for Collective Navigation of Robotic Swarms
Source: arXiv:2202.01141 source file (2022-09-11)
Supplement: Supplementary file 1 [file appendix.tex]

%\newpage
\section{APPENDIX}

\begin{algorithm}
\SetAlgoLined
%\KwResult{Write here the result }
Randomly initialise $N$ critic neural networks, $Q_{1, ... , N}(s, a|\theta^Q_{1, ... , N})$ and $N$ actor neural networks $\pi_{1, ... , N}(s|\theta_{1, ... , N}^{\pi})$ with weights $\theta_{1, ... , N}^{Q}$ and $\theta_{1, ... , N}^{\pi}$\\
Initialise $N$ target networks $Q_{1, ... , N}^\prime$ and $\pi_{1, ... , N}^\prime$ with weights $\theta_{1, ... , N}^{Q^\prime}$ $\leftarrow$ $\theta_{1, ... , N}^Q$, $\theta_{1, ... , N}^{\pi^\prime}$ $\leftarrow$ $\theta_{1, ... , N}^{\pi}$\\
Initialise local memories $R_{1, ... , N}$\\
\For{episode = 1, $...$, M}
{ Initialise the states $s_t = s_1$\\
\For{t = 1, $...$, T}{
Run $N$ actors and collect transition samples $D_t$ = ($s_t, a_t, r_t, s_{t+1}$) into the local memories $R_{1, ... , N}$ \\

  \If{t = 0 mod $t_{train}$}
  {Sample $l$ transitions ($s_i, a_i, r_i, s_{i+1}$) from the local memories, $R_{1, ... , N}$\\
  Set $y_i = r_i + \gamma Q^{\prime}(s_i, \pi^{\prime}(s_{i+1}|\theta^{\pi^\prime})|\theta^{Q^\prime})$\\
  
  Update critic network by minimizing the loss: $L_Q = \frac{1}{N}\sum_i(y_i-Q(s_i,a_i|\theta^Q))^2$\\
  Update actor network using the sampled policy gradient:
  $\nabla_{\theta^\pi}J \approx \frac{1}{N}\sum_i \nabla_a Q(s,a|\theta^{Q})|_{s=s_i, a=\pi(s_i)} \par \quad\quad\quad\quad \cdot\nabla_{\theta^\pi}\pi(s_i|\theta^\pi)|_{s=s_i}$\\}
  \If {t = 0 mod $t_{target}$}{Update the target networks: $\theta^{Q^\prime} \leftarrow \theta^Q$,$ \theta^{\pi^\prime} \leftarrow \theta^{\pi}$}
 }
 }
 \caption{Independent DDPG (IDDPG)}
 \label{algo:IDDPG}
\end{algorithm}

\begin{algorithm}
\SetAlgoLined
%\KwResult{Write here the result }
Randomly initialise a critic neural network, $Q(s, a|\theta^Q)$ and an actor neural network $\pi(s|\theta^{\pi})$ with weights $\theta^{Q}$ and $\theta^{\pi}$\\
Initialise target networks $Q^\prime$ and $\pi^\prime$ with weights $\theta^{Q^\prime}$ $\leftarrow$ $\theta^Q$, $\theta^{\pi^\prime}$ $\leftarrow$ $\theta^{\pi}$\\
Initialise a shared memory $R$\\
\For{\text{episode = 1, $...$, M}}
{Initialise the states $s_t = s_1$ for $N$ robots\\
\For{\text{t = 1, $...$, T}}{
Run $N$ robots and collect transition samples $D_t$ = ($s_t, a_t, r_t, s_{t+1}$) into the shared memory, $R$\\

  \If{t = 0 mod $t_{train}$}
  {Sample $N$ transitions ($s_i, a_i, r_i, s_{i+1}$) from the shard memory, $R$\\
  Set $y_i = r_i + \gamma Q^{\prime}(s_i, \pi^{\prime}(s_{i+1}|\theta^{\pi^\prime})|\theta^{Q^\prime})$\\
  
  Update the critic network by minimizing the loss: $L_Q = \frac{1}{N}\sum_i(y_i-Q(s_i,a_i|\theta^Q))^2$\\
  Update the actor network using the sampled policy gradient:
  $\nabla_{\theta^\pi}J \approx \frac{1}{N}\sum_i \nabla_a Q(s,a|\theta^{Q})|_{s=s_i, a=\pi(s_i)} \par \quad\quad\quad\quad \cdot\nabla_{\theta^\pi}\pi(s_i|\theta^\pi)|_{s=s_i}$\\}
  \If {t = 0 mod $t_{target}$}{Update the target networks: $\theta^{Q^\prime} \leftarrow \theta^Q$,$ \theta^{\pi^\prime} \leftarrow \theta^{\pi}$}
 }
 }
 \caption{Shared Network DDPG (SNDDPG)}
 \label{algo:SNDDPG}
\end{algorithm}

\begin{algorithm}
\SetAlgoLined
%\KwResult{Write here the result }
Randomly initialise $N$ critic neural networks, $Q_{1, ... , N}(s, a|\theta^Q_{1, ... , N})$ and $N$ actor neural networks $\pi_{1, ... , N}(s|\theta_{1, ... , N}^{\pi})$ with weights $\theta_{1, ... , N}^{Q}$ and $\theta_{1, ... , N}^{\pi}$\\
Initialise $N$ target networks $Q_{1, ... , N}^\prime$ and $\pi_{1, ... , N}^\prime$ with weights $\theta_{1, ... , N}^{Q^\prime}$ $\leftarrow$ $\theta_{1, ... , N}^Q$, $\theta_{1, ... , N}^{\pi^\prime}$ $\leftarrow$ $\theta_{1, ... , N}^{\pi}$\\
Initialise a shared memory $R_{1, ... , N}$\\
\For{episode = 1, $...$, M}
{ Initialise the states $s_t = s_1$\\
\For{t = 1, $...$, T}{
Run $N$ robots and collect transition samples $D_t$ = ($s_t, a_t, r_t, s_{t+1}$) into the shared memory $R$ \\

  \If{t = 0 mod $t_{train}$}
  {Sample $l$ transitions ($s_i, a_i, r_i, s_{i+1}$) from the shared memory, $R$\\
  Set $y_i = r_i + \gamma Q^{\prime}(s_i, \pi^{\prime}(s_{i+1}|\theta^{\pi^\prime})|\theta^{Q^\prime})$\\

  Update critic network by minimizing the loss: $L_Q = \frac{1}{N}\sum_i(y_i-Q(s_i,a_i|\theta^Q))^2$\\
  Update actor network using the sampled policy gradient:
  $\nabla_{\theta^\pi}J \approx \frac{1}{N}\sum_i \nabla_a Q(s,a|\theta^{Q})|_{s=s_i, a=\pi(s_i)} \par \quad\quad\quad\quad \cdot\nabla_{\theta^\pi}\pi(s_i|\theta^\pi)|_{s=s_i}$\\}
  \If {t = 0 mod $t_{target}$}{Update the target networks: $\theta^{Q^\prime} \leftarrow \theta^Q$,$ \theta^{\pi^\prime} \leftarrow \theta^{\pi}$}
 }
 }
 \caption{Shared Experience DDPG (SEDDPG)}
 \label{algo:SEDDPG}
\end{algorithm}
